# Supplementary material for: Simple Cues Lead to a Strong Multi-Object Tracker
Source: arXiv:2206.04656 source file (2023-04-26)
Supplement: Supplementary file 3 [file ablations_proxies.tex]

\begin{table*}[hbt!]

\centering
\resizebox{0.9\textwidth}{!}{
\begin{tabular}{@{}l|ccc|ccc|ccc|ccc@{}}
\hline
 & \multicolumn{3}{c|}{MOT17} & \multicolumn{3}{c|}{MOT20} & \multicolumn{3}{c|}{Dance} & \multicolumn{3}{c}{BDD} \\
 \hline
 & \textbf{HOTA} $\uparrow$ &  \textbf{IDF1} $\uparrow$ & \textbf{MOTA} $\uparrow$ & \textbf{HOTA} $\uparrow$ & \textbf{IDF1} $\uparrow$ &  \textbf{MOTA} $\uparrow$ & \textbf{HOTA} $\uparrow$ &  \textbf{IDF1} $\uparrow$ & \textbf{MOTA} $\uparrow$ & \textbf{HOTA} $\uparrow$ & \textbf{IDF1} $\uparrow$ &  \textbf{MOTA} $\uparrow$ \\
\hline
Our Proxy & 63.1 & 74.4 & 69.7 & 63.6& 75.6  & 69.7 \\
\hline
Mean Features &  \\ 
Mode Features &  \\ 
Median Features &  \\ 
Moving Average Features &  \\ 
\hline
 \end{tabular}}

\caption{Comparison of different proxy generation methods.}
\label{tab:proxy_ablations}
\end{table*}
